# Supplementary material for: Frequency-Selective Beamforming Cancellation Design for Millimeter-Wave Full-Duplex
Source: arXiv:1910.11983 source file (2019-10-26)
Supplement: Supplementary file 1 [file eq-si-channel-los.tex]

\begin{align} \label{eq:si-channel-los}
	\left[\channel^{\textrm{LOS}}_{ii}\right]_{m,n} &= \frac{\rho}{r_{m,n}}\exp \left(-\j 2 \pi \frac{r_{m,n}}{\lambda_{c}} \right)
\end{align}
